# Supplementary material for: In vivo anomalous diffusion and weak ergodicity breaking of lipid granules
Source: arXiv:1010.0347 source file (2011-01-17)
Supplement: Supplementary file 1 [file supplementary.pdf]

# Supplementary Material to In vivo anomalous diffusion and weak ergodicity breaking of lipid granules

Jae-Hyung Jeon,[1] Vincent Tejedor,[2] Stas Burov,[3] Eli Barkai,[3] Christine Selhuber-Unkel,[4,5] Kirstine Berg-Sørensen,[6] Lene Oddershede,[5] and Ralf Metzler[1]

[1]*Physics Department T30g, Technical University of Munich, 85747 Garching, Germany*
[2]*Physique Théorique de la matiére condensée, Université Pierre et Marie Curie, 4 place Jussieu, 75252 Paris, France*
[3]*Physics Department, Bar-Ilan University, Ramat Gan 52900, Israel*
[4]*Institute for Materials Science, University of Kiel, Kaiserstraße 2, 24143 Kiel, Germany*
[5]*Niels Bohr Institute, Blegdamsvej 17, 2100 København Ø, Denmark*
[6]*Physics Department, Technical University of Denmark, 2800 Kongens Lyngby, Denmark*

We here detail the preparation of *S.pombe* cells and the microscopic methods used to track the lipid granules. Moreover we present some additional Figures, corroborating the quantitative statements in the main article. The numbering of the Figures is consecutive with the numbers in the main article.

## MATERIALS AND METHODS

### Cell preparation

We used fission yeast cells (*S.pombe*, D817) expressing a GFP-fused marker of the nuclear and plasma membrane systems [D. Q. Ding et al., Genes to Cells **5**, 169 (2000).]. When the cells are in interphase, their length is approximately 12 $\mu$m and their width 4 $\mu$m. Spherical lipid granules, about 300 nm in diameter, are endogenously present in the cytoplasm of these cells [C. F. Robinow and J. S. Hyams, in Molecular Biology of the Fission Yeast (Academic Press, New York, NY, 1989), pp. 273-330]. These granules are sufficiently refractive to be visualized with bright-field microscopy. Note that lipid granules were previously used as endogenous tracers [S. Yamada, D. Wirtz, and S. C. Kuo, Biophys. J. **78**, 1736 (2000); S. S. Rogers, T. A. Waigh, and J. R. Lu, *ibid.* **94**, 3313 (2008)].

The cells were cultured on AA-Leu agar plates for 12-14 h at 33° C and after growth stored at 4° C. Prior to the experiments the cells were suspended into liquid AA-Leu medium.

The fluid chamber for the experiments consisted of two glass slides glued together by a layer of double sticky tape as a spacer. The chamber was then filled with the cell suspension. The cells were allowed to relax on the surface for approx. 20 minutes, so that they do not move during data acquisition. The experiments were performed at room temperature (22–24° C).

### Optical tweezers tracking

Optical tweezers were created using a Nd:YVO4 laser (5W Spectra Physics BL-106C, $\lambda = 1064$ nm, $\text{TEM}_{00}$), implemented in an inverted fluorescence microscope (Leica, DMI 6000) equipped with a cooled CCD camera (Andor, Ixon cooled EMCCD). We used an oil immersion objective from Leica (HCX PL Apo, 100/NA=1.4 oil Cs). The forward scattered light of the highly-refractive intracellular granules was recorded by a silicon quadrant photodiode (S5981, Hamamatsu) in the back focal plane, allowing nanometer precision detection of the granule position in the laser focus. The motion of a single granule in the laser focus was tracked for approximately 3 sec at a sampling frequency of 22 kHz. We used a laser power of approximately 0.05 W at the sample, rendering this technique nearly non-invasive. The voltage signal from the photodiode was digitalized using home-written Labview algorithms. While the voltage signal is directly proportional to the particle position with respect to the trap center, due to lack of knowledge of the precise optical conditions in the cell we could not convert the voltage signal to absolute distance. The time averaged mean squared displacement obtained from this method is therefore given in arbitrary units.

We note that during the optical tweezers tracking the granule particles become increasingly confined in the optical tweezers' trapping potential. The time averaged mean squared displacement of an ergodic process would therefore saturate to a stationary value. CTRW subdiffusion, as shown in our data, is non-stationary and shows a power-law growth of the time averaged mean squared displacement.

### Single particle tracking

At longer times the motion of granules in the cell was detected by video-based image analysis. Bright-field microscopy imaging was carried out on a Leica DMIRE2 microscope, using an oil immersion objective (Leica PL Apo 100x), an AVT Pike F100B camera (Allied Vision Technologies), and SmartView software (Allied Vision Technologies) for recording. To confirm that the cells were in interphase, the GFP fluorescence of the membranes was observed. Particle tracking was carried out using an algorithm by Rogers et al. [S. S. Rogers et al., Phys. Biol.

4, 220 (2007)]. This algorithm is well-established for intracellular granule tacking [S. S. Rogers, T. A. Waigh, and J. R. Lu, Biophys. J. **94**, 3313 (2008)].

## ANOMALOUS DIFFUSION PROCESSES

Both CTRW and FBM give rise to an ensemble averaged mean squared displacement of the form (1). However, they are fundamentally different processes, as outlined here.

### Continuous time random walk

Every step in a CTRW is characterised by a random jump length and a random waiting time passing before the following step. Jump lengths and waiting times are chosen independently. CTRWs are therefore renewal processes. For subdiffusion we assume that the variance of the jump lengths converges, $\langle\delta x^2\rangle < \infty$. For instance, on a lattice with spacing $a$, we have $\langle\delta x^2\rangle = a^2$. For unbiased diffusion considered here, the average first moment of the jump length distribution vanishes, $\langle\delta x\rangle = 0$. The distribution of waiting times $t$, however, is chosen in the inverse power-law form

$$\psi(t) \simeq \frac{\tau^\alpha}{t^{1+\alpha}} \tag{1}$$

for large $t$, where $0 < \alpha < 1$. This is scale-free form causes a divergence of the mean waiting time, $\langle t\rangle \to \infty$, giving rise to effects such as ageing [1, 2] and weak ergodicity breaking [3]. In Eq. (1), the quantity $\tau$ is a scaling factor. The anomalous diffusion constant reads $K_\alpha = \langle\delta x^2\rangle/[2\tau^\alpha]$ [4, 5].

Due to the scale-freeness of $\psi(t)$ individual waiting times $t$ can become quite large. Even in very long time series, individual $t$ may become of the order of the overall process time. Typically, due to the divergence of the characteristicwaiting time, also mean first passage times diverge, even in finite geometries. This property sets CTRW subdiffusion apart from FBM. Power-law waiting time distributions with a cutoff time $\tau^*$ eventually converge to normally diffusive motion, with finite mean first passage times.

CTRW has become a standard statistical tool to describe processes ranging from charge carrier motion in amorphous semiconductors [6], over the tracer motion in groundwater [7], to the particle motion in actin networks [8]. In the latter the tracer particles of size 250 nm experience multiple trapping events in the cage-like structure of the semiflexible polymer network, such that repeated escapes from single cages gives rise to a power-law form (1) of the emanating waiting time distribution. Particularly, the resulting anomalous diffusion exponent $\alpha$ in these experiments depends on the ratio of tracer particle size and typical mesh size of the actin network.

### Fractional Brownian motion

FBM is a stochastic process, whose position is governed by the Langevin equation

$$\frac{dx(t)}{dt} = \xi(t), \tag{2}$$

or, alternatively, by $x(t) = \int_0^t \xi(t')dt'$. The motion is driven by stationary, fractional Gaussian noise $\xi(t)$ with zero mean $\langle\xi(t)\rangle$ and long-ranged noise correlation [9]

$$\begin{aligned}\langle\xi(t_1)\xi(t_2)\rangle &= \alpha K_\alpha^*(\alpha-1)|t_1-t_2|^{\alpha-2}\\ &+2\alpha K_\alpha^*|t_1-t_2|^{\alpha-1}\delta(t_1-t_2).\end{aligned} \tag{3}$$

This form contrasts the uncorrelated noise for normal diffusion $\alpha = 1$: $\langle\xi(t_1)\xi(t_2)\rangle = 2K_1\delta(t_1-t_2)$. The exponent $\alpha$ chosen here relates to the traditionally used Hurst exponent by $H = \alpha/2$. In subdiffusive processes the fractional Gaussian noise is anticorrelated, with asymptotic behavior $\langle\xi(t_1)\xi(t_2)\rangle \sim -K_\alpha^*\alpha|\alpha-1||t_1-t_2|^{\alpha-2}$. Any given step is therefore likely to direct oppositely to the previous step. The position autocorrelation function of FBM becomes

$$\langle x(t_1)x(t_2)\rangle = K_\alpha^*\Big(t_1^\alpha + t_2^\alpha - |t_1-t_2|^\alpha\Big), \tag{4}$$

so that at equal times $t_1 = t_2$ we recover the mean squared displacement (1).

If the fractional Gaussian noise is not considered external, but subject to the fluctuation-dissipation theorem, the generalised Langevin equation (GLE) [10] describes the motion,

$$m\frac{d^2x(t)}{dt^2} = -\overline{\gamma}\int_0^t (t-t')^{\beta-2}\frac{dx}{dt'}dt' + \eta\xi(t), \tag{5}$$

where we write $\beta$ instead of the exponent $\alpha$ in Eq. (3). In Eq. (5), we define the coupling coefficient $\eta = \sqrt{k_B\mathcal{T}\overline{\gamma}/[\beta K_\beta^*(\beta-1)]}$ according to the fluctuation-dissipation theorem, where $k_B\mathcal{T}$ is the thermal energy. We only consider the overdamped limit, in which the inertia term $md^2x(t)/dt^2$ becomes negligible. The GLE then produces the mean squared displacement

$$\langle x^2(t)\rangle \simeq t^{2-\beta}. \tag{6}$$

In contrast to FBM, that is, the GLE leads to subdiffusion for persistent noise with $1 < \beta < 2$, while $0 < \beta < 1$ yields superdiffusion.

FBM and the related GLE are used to describe processes such as long term storage capacity of water reservoirs [11], climate fluctuations [12], economical market

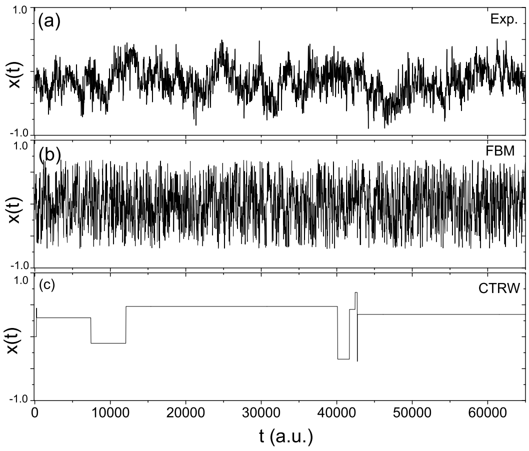


Figure 5: Time series $x(t)$ of the experimentally recorded granule motion (a), and from simulations of FBM (b) and CTRW [note the pronounced stalling events] (c) with $\alpha = 0.2$.

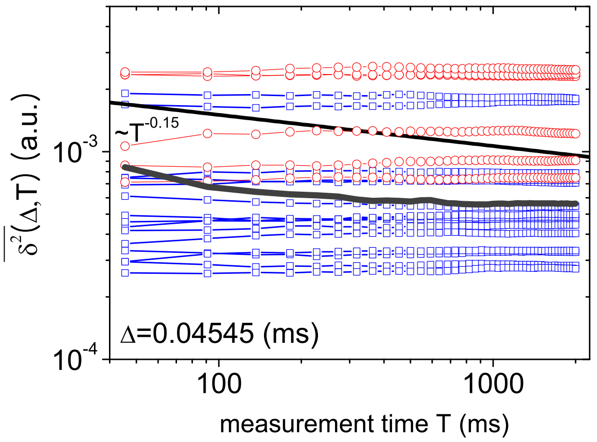


Figure 6: Ageing plot: Both for cells in early telophase (blue, □) and early mitotic phase (red, ◯) no significant dependence on the measurement time $T$ is observed, i.e., no ageing occurs, in contrast to the prediction $\simeq T^{\alpha-1}$ for CTRW subdiffusion with scale-free power-law waiting time distribution corresponding to $\tau^* \to \infty$ (black —). The wide grey line shows the expected behavior of CTRW subdiffusion with waiting time cutoff, Eq. (3). As parameters we used $\alpha = 0.85$, $\tau^* = 182$ msec, $\tau = 0.04545$ msec, and $T = 3.0$ sec.

dynamics [13], single file diffusion [14], and elastic models [15]. Motion of this type has also been associated with the relative motion of aminoacids in proteins [16], and the free diffusion of biopolymers under molecular crowding conditions [17, 18].

## ADDITIONAL FIGURES

Below we present some additional Figures, that are referred to in the main text. We here give a brief summary of these Figures.

Fig. 5a shows a typical time series of the granule motion, as observed by indirect optical tweezers recording. Qualitatively this behavior is not significantly different from Brownian motion. In Fig. 5b and c we show simulations results for subdiffusive FBM and CTRW with an exponent $\alpha = 0.2$, corresponding to the slope in the second power-law region of Fig. 1 in the main text. Clearly, panels b and c display completely different behavior compared to panel a: subdiffusive FBM is much more erratic, mirroring the highly antipersistent character of fractional Gaussian noise. In contrast, subdiffusive CTRW with such a low value for the anomalous diffusion exponent displays very pronounced stalling events. These observations underline that the second power-law region $\overline{\delta^2(\Delta, T)} \simeq \Delta^\beta$ with $\beta \approx 0.15 \ldots 0.20$ in the short time data of the granule motion are inconsistent with anomalous motion corresponding to an ensemble averaged mean squared displacement $\langle \mathbf{r}^2(t) \rangle \simeq t^{0.15\ldots0.20}$.

Fig. 6 demonstrates the absence of ageing in the time series for lipid granule motion in *S.pombe* cells, in both cell stages. The full black line shows the ageing effect with the overall measurement time $T$ predicted for a CTRW process with power-law waiting time distribution in absence of a cutoff. The dark grey line depicts the simulated behavior for CTRW with cutoff, showing only very reduced variation for short $T$. Similar behavior is observed at different lag times.

In Fig. 7 we show the scatter distribution $\phi(\xi)$ corresponding to Fig. 2, at longer lag times, $\Delta = 4.545$ msec and $\Delta = 45.45$ msec. CTRW subdiffusion with cutoff time $\tau^* = 182$ msec describes well the observed behaviour.

Fig. 8 shows the distribution $\phi(\xi)$ for the motion of the lipid granules in *S.pombe* at longer times, measured directly by video imaging. The corresponding ageing plot of $\overline{\delta^2(\Delta, T)}$ as function of the measurement time $T$ does not exhibit any features of ageing. The cells in the long time measurements were all in interphase.

Fig. 9 for the video tracking data shows the ratios $\langle r^4(t) \rangle / \langle r^2(t) \rangle^2$ for regular moments and $\langle r^4(t) \rangle_{\max} / \langle r^2(t) \rangle^2_{\max}$ for the mean maximal excursion statistics developed in V. Tejedor et al., Biophys. J. **98**, 1364 (2010). The data are consistent with FBM. Here, $r(t) = \sqrt{x^2(t) + y^2(t)}$.

In Fig. 10 we show three individual trajectories measured by video tracking at longer times. The top panel shows typical behavior with strong antipersistence. In the middle a weak drift appears. At the bottom we see a trajectory with strong average displacement over the measured range. Here, likely active biological effects come into play. The inset demonstrates that the antiper-

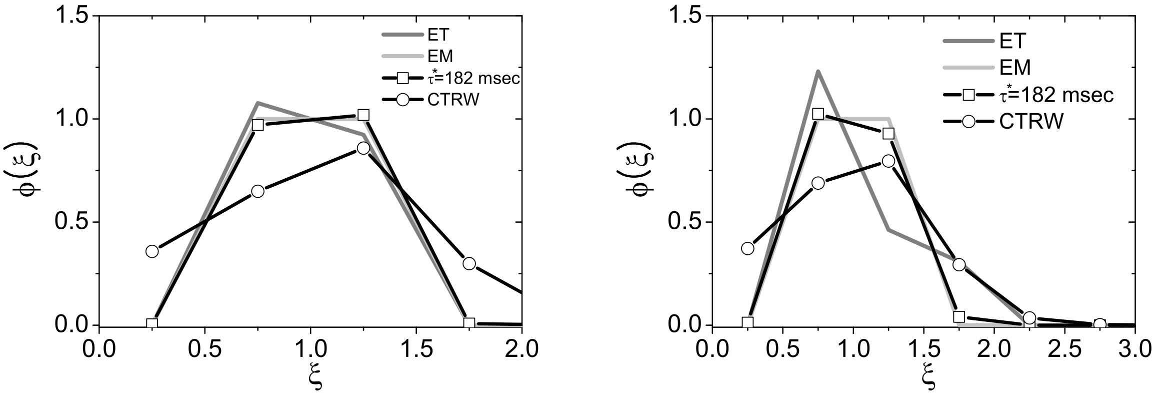


Figure 7: Scatter plot comparing the behaviour measured at Early Telophase and Early Mitosis at $\Delta = 4.545$ msec (Left) and $\Delta = 45.45$ msec (Right) with the predicted shapes of CTRW subdiffusion with cutoff time $\tau^* = 182$ msec, $\alpha = 0.85$, $\tau = 0.04545$ msec, and $T = 3.0$ sec. The cutoff CTRW provides an excellent description of the data, while the scale-free CTRW without cutoff shows deviations, especially at $\xi = 0$.

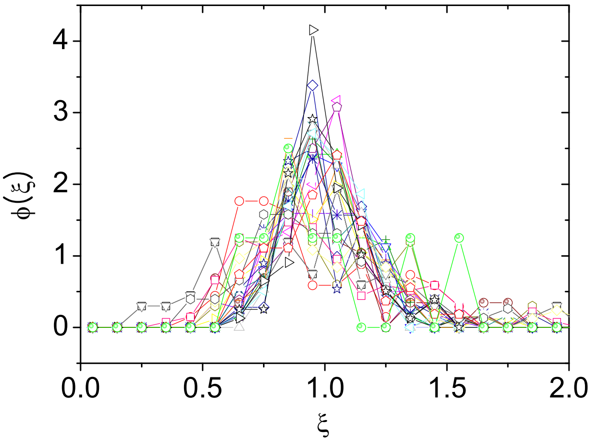


Figure 8: Scatter distribution $\phi(\xi)$ for the long time granule motion in *S.pombe* yeast cells. A bell-shaped curve is observed. The curves are evaluated for a lag time of the length of the frame interval, such that $\Delta \approx 0.01$ sec.

sistent behavior is still visible.

Finally, Fig. 11 displays the velocity-velocity correlation $C_v^{(\varepsilon)}(\Delta)/C_v^{(\varepsilon)}(0)$ functions for the long time motion of the lipid granules [for a definition of $C_v^{(\varepsilon)}(\Delta)$, see S. Weber et al, Phys. Rev. Lett. **104**, 238102 (2010)]. Here, $\varepsilon$ is the time interval defining a velocity through $v^{(\varepsilon)}(t) = r(t+\varepsilon) - r(t)$. The analysis shows that the observed behavior is consistent with both CTRW and FBM subdiffusion under confinement. For details on the velocity autocorrelation functions, see S. Burov, J.-H. Jeon, R. Metzler, and E. Barkai, E-print arXiv:1009.4846.

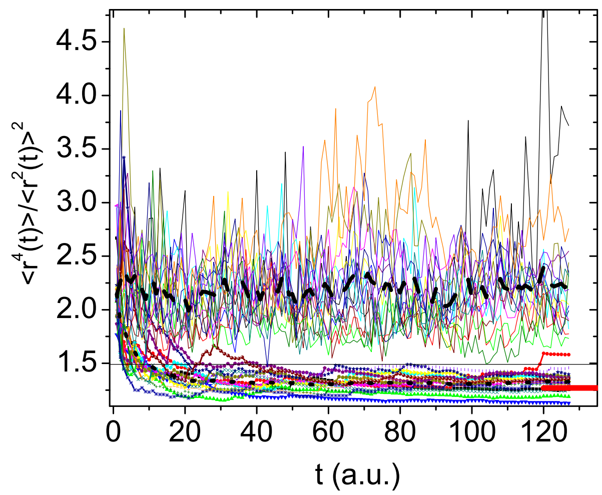


Figure 9: Moment ratios $\langle r^4(t)\rangle/\langle r^2(t)\rangle^2$ for regular moments and $\langle r^4(t)\rangle_{\max}/\langle r^2(t)\rangle^2_{\max}$ for the mean maximal excursion statistics [V. Tejedor et al., Biophys. J. **98**, 1364 (2010)]. The respective mean is shown by the thick black dashed and dotted lines. The bars on the right represent the theoretical values for FBM with $\alpha = 0.80 \ldots 0.85$. The good agreement supports that the motion is indeed governed by FBM.

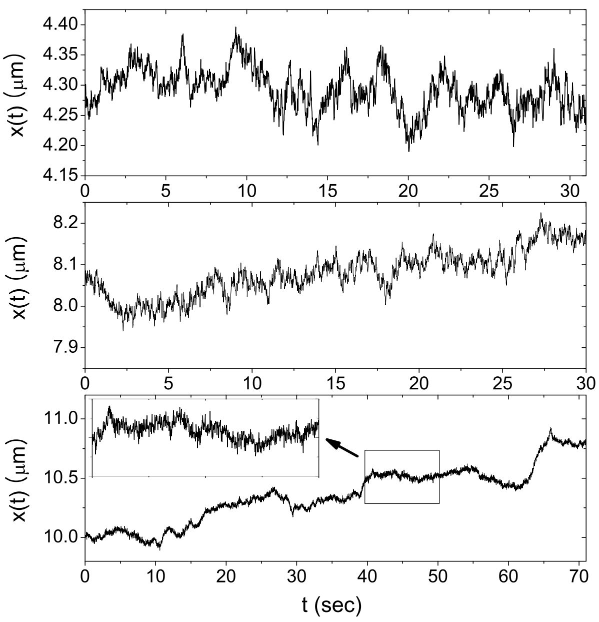


Figure 10: Sample trajectories of lipid granule particles measured by video tracking at longer times. Top: typical trajectory with apparent antipersistent motin. Middle: Motion with some apparent bias. Bottom: Strong bias effecting a nonzero average first moment, possibly reflecting active biological processes. The inset indicates the antipersistence of the trajectory.

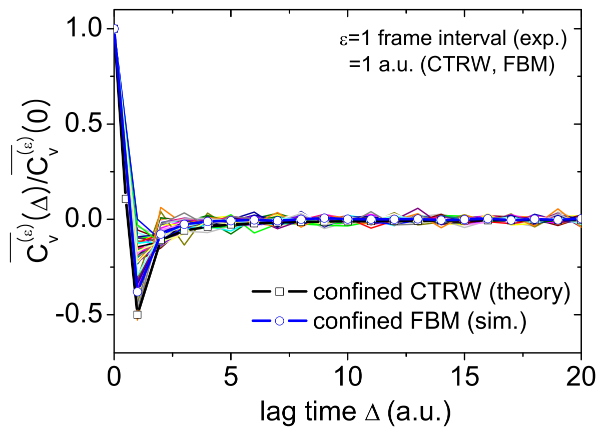


Figure 11: Velocity autocorrelation function for the long time data (colored lines). The experimental behavior is consistent with both the theoretical prediction for confined CTRW subdiffusion and the simulations results for confined FBM.

[1] C. Monthus and J.-P. Bouchaud, J. Phys. A **29**, 3847 (1996); G. Ben Arous, A. Bovier, and V. Gayrard Phys. Rev. Lett. **88**, 087201 (2002)
[2] E. Barkai and Y. C. Cheng, J. Chem. Phys. **118**, 6167 (2003).
[3] J.-P. Bouchaud, J. Phys. (Paris) I, **2**, 1705 (1992); G. Bel and E. Barkai, Phys. Rev. Lett. **94**, 240602 (2005); A. Rebenshtok and E. Barkai, *ibid.* **99**, 210601 (2007); M. A. Lomholt, I. M. Zaid, and R. Metzler, *ibid.*, 98, 200603 (2007); I. M. Zaid, M. A. Lomholt, and R. Metzler, Biophys. J. **97**, 710 (2009); G. Aquino, P. Grigolini, and B. J. West, EPL **80**, 10002 (2007).
[4] R. Metzler and J. Klafter, Phys. Rep. **339**, 1 (2000); J. Phys. A **37**, R161 (2004); E. Barkai, Phys. Rev. E **63**, 046118 (2001).
[5] R. Metzler, E. Barkai, and J. Klafter, Phys. Rev. Lett. **82**, 3563 (1999); Europhys. Lett. **46**, 431 (1999). E. Barkai, R. Metzler, and J. Klafter, Phys. Rev. E **61**, 132 (2000); R. Metzler, J. Klafter, and I. M. Sokolov, *ibid.* **58**, 1621 (1998).
[6] H. Scher and E. W. Montroll, Phys. Rev. B **12**, 2455 (1975).
[7] H. Scher, G. Margolin, R. Metzler, J. Klafter, and B. Berkowitz, Geophys. Res. Lett. **29**, 1061 (2002); B. Berkowitz, A. Cortis, M. Dentz and H. Scher, Reviews of Geophysics, 44, RG2003 (2006).
[8] I. Y. Wong, M. L. Gardel, D. R. Reichman, E. R. Weeks, M. T. Valentine, A. R. Bausch, and D. A. Weitz, Phys. Rev. Lett. **92**, 178101 (2004).
[9] A. N. Kolmogorov, Dokl. Acad. Sci. USSR **26**, 115 (1940); B. B. Mandelbrot and J. W. van Ness, SIAM Rev. **1**, 422 (1968); H. Qian, Fractional Brownian Motion and Fractional Gaussian Noise. In G. Rangarajan and M.Z. Ding (eds), *Processes with Long-Range Correlations* (Springer, Lecture Notes in Physics, Vol.621), pp.22-33.
[10] R. Kubo, M. Toda, and N. Hashitsume, Statistical Physics II: Nonequilibrium Statistical Mechanics (Springer-Verlag, Heidelberg, 1995).
[11] H. E. Hurst, Trans. Am. Soc. Civ. Eng. **116**, 400 (1951).
[12] T. N. Palmer, G. J. Shutts, R. Hagedorn, F. J. Doblas-Reyes, T. Jung, and M. Leutbecher, Annu. Rev. Earth Planet Sci. **33**, 163 (2005).
[13] I. Simonsen, Physica A **322**, 597 (2003); N. E. Frangos, S. D. Vrontos, and A. N. Yannacopoulos, Appl. Stoch., Models Bus. Ind. **23**, 403 (2007).
[14] T. E. Harris, J. Appl. Probab. **2**, 323 (1965); L. Lizana and T. Ambjörnsson, Phys. Rev. Lett. **100**, 200601 (2008); L. Lizana, T. Ambjörnsson, A. Taloni, E. Barkai, and M. A. Lomholt, Phys. Rev. E **81**, 051118 (2010); E. Barkai and R. Silbey, Phys. Rev. Lett. **102**, 050602 (2009).
[15] A. Taloni, A. V. Chechkin, and J. Klafter, Phys. Rev. Lett. **104**, 160602 (2010).
[16] S.C. Kou and X. S. Xie, Phys. Rev. Lett. **93**, 180603 (2004); W. Min, G. Luo, B. J. Cherayil1, S. C. Kou, and X. S. Xie, Phys. Rev. Lett. **94**, 198302 (2005).
[17] J. Szymanski and M. Weiss, Phys. Rev. Lett. **103**, 038102 (2009).
[18] S. C. Weber, A. J. Spakowitz, and J. A. Theriot, Phys. Rev. Lett. **104**, 238102 (2010).
